# Supplementary material for: Ensemble Distribution Distillation
Source: arXiv:1905.00076 source file (2019-11-25)
Supplement: Supplementary file 1 [file appendix_nll.tex]

\section{Negative log-likelihood and Calibration}\label{apn:calibration}

In this work, measures of uncertainty derived from ensembles, EnD and EnD$^2$ models were assessed on threshold-based outlier detection tasks, such as misclassification detection/rejection and out-of-distribution input detection. These tasks assess measures of uncertainty on a \emph{per-prediction} basis on a downstream application. However, it is also possible to assess measures of uncertainty on a \emph{per-dataset} basis by considering metrics like the test-set negative log-likelihood (NLL) and calibration \citep{swag}. However, as these metrics are removed from downstream applications, they are not considered in the main paper and instead provided in this appendix. Nevertheless, it is known that ensembles yield improvements in calibration and test-set negative log-likelihood \citep{deepensemble2017}, and it is therefore interesting to assess whether EnD and EnD$^2$ models retain those improvements. 

Table~\ref{tab:nll-cifar-res} shows the results for negative log-likelihood and calibration. Both Ensemble Distillation and Ensemble Distribution Distillation seem to give similarly minor gains in NLL over a single model. However, EnD seems to have marginally better NLL performance, while EnD$^2$ tends to yield better calibration performance. There are seemingly limited gains in ECE and NLL when using auxiliary data during distillation for EnD$^2$, and sometimes even a degradation in NLL and ECE. This may be due to a Dirichlet output distribution attempting to capture non-Dirichlet-distributed ensemble predictions on the auxiliary data. Furthermore, metrics like ECE and NLL are evaluated on in-domain data, which would explain the lack of improvement from distilling ensemble behaviour on auxiliary data.
\begin{table}[htb!]
\caption{Mean test-set negative log-likelihood (NLL) and expected calibration error (ECE) on C10/C100/TIM across three models $\pm2\sigma$.}\label{tab:nll-cifar-res}
\centering
\begin{tabular}{ll|rr|rr|rr}
\toprule
Dataset   & Criterion & Individual                & Ensemble & EnD & EnD$^2$ & EnD$_{\tt +AUX}$  &  EnD$^2_{\tt +AUX}$ \\
\midrule
\multirow{2}{*}{C10} & NLL &  0.25 \scriptsize{$\pm 0.01 $} & \textbf{0.19}  \scriptsize{$\pm$ NA} & 0.22 \scriptsize{$\pm 0.01 $} & 0.25 \scriptsize{$\pm 0.01 $} & 0.22 \scriptsize{$\pm 0.01 $}  &  0.24 \scriptsize{$\pm 0.00 $} \\
& ECE & 2.2 \scriptsize{$\pm 0.4 $} & 1.3  \scriptsize{$\pm$ NA} &  2.6 \scriptsize{$\pm 0.2$}  &  \textbf{1.0 \scriptsize{$\pm 0.2$}} & 2.6 \scriptsize{$\pm 0.6 $} & 2.2  \scriptsize{$\pm 0.4$}\\
\midrule
\multirow{2}{*}{C100} & NLL  &  1.16 \scriptsize{$\pm 0.03 $} &  \textbf{0.88}  \scriptsize{$\pm $ NA} &  1.06 \scriptsize{$\pm 0.01$} &  1.14  \scriptsize{$\pm 0.01$} & 0.98  \scriptsize{$\pm 0.00$} & 1.14 \scriptsize{$\pm 0.01$}\\
& ECE & 9.3 \scriptsize{$\pm 0.8$} & \textbf{1.2}   \scriptsize{$\pm $ NA} &  8.2 \scriptsize{$\pm 0.3$} &   4.9 \scriptsize{$\pm 0.5$} & 1.9 \scriptsize{$\pm 0.3$} & 5.6 \scriptsize{$\pm 0.5$}\\
\midrule
\multirow{2}{*}{TIM} & NLL  &  2.15 \scriptsize{$\pm 0.05 $} & \textbf{1.51}   \scriptsize{$\pm $ NA} &  1.77 \scriptsize{$\pm 0.01$} &   1.83 \scriptsize{$\pm 0.02$} & 1.78 \scriptsize{$\pm 0.01$} & 1.84 \scriptsize{$\pm 0.02$}\\
& ECE & 18.3 \scriptsize{$\pm 0.8$} & \textbf{3.8}  \scriptsize{$\pm $ NA} & 14.8 \scriptsize{$\pm 0.4 $} &   7.2 \scriptsize{$\pm 0.4 $} & 14.9 \scriptsize{$\pm 0.3 $}  & 7.2 \scriptsize{$\pm 0.2 $}\\
\bottomrule
\end{tabular}
\end{table}
