# Supplementary material for: Ensemble Distribution Distillation
Source: arXiv:1905.00076 source file (2019-11-25)
Supplement: Supplementary file 2 [file ensemble_analysis.tex]

\begin{table}[htb!]
\caption{Mean test-set negative log-likelihood (NLL) and expected calibration error (ECE) on C10/C100/TIM across three models $\pm2\sigma$.}\label{tab:nll-cifar-res}
\centering
\begin{tabular}{ll|cc|cc}
\toprule
\multirow{2}{*}{Dataset}   & \multirow{2}{*}{Architecture} & \multicolumn{2}{c}{Individual} & \multicolumn{2}{c}{Ensemble} \\
&                            & Train Error & Test Error & Train Error & Test Error \\
\midrule
\multirow{2}{*}{C10} & VGG16 & 2.8 & 8.0 & 1.7 & 6.2 \\ 
                     & RN34  & 0.0 & 4.3 & 0.0 & 3.2 \\ 
\midrule
\multirow{2}{*}{C100} & VGG16 & 15.2 & 30.4 & 11.3 & 26.3 \\ 
                     & RN34   & 0.0 & 21.8 & 0.0  & 17.6 \\ 
\midrule
\multirow{2}{*}{TIM} & VGG16 & 4.1 & 41.8 & 1.4 & 36.6\\ 
                     & RN34  & 0.0 & 36.7 & 0.0 & 28.9\\ 
\bottomrule
\end{tabular}
\end{table}

\begin{figure}[ht!]
     \centering
     \begin{subfigure}[b]{0.321\textwidth}
         \centering
         \includegraphics[width=0.94\textwidth]{figures/C10_VGG_ensemble.png}
         \caption{CIFAR-10 VGG Ensemble}
     \end{subfigure}
     \hfill
     \begin{subfigure}[b]{0.32\textwidth}
         \centering
         \includegraphics[width=0.94\textwidth]{figures/C100_VGG_ensemble.png}
         \caption{CIFAR-100 VGG Ensemble}
     \end{subfigure}
     \hfill
     \begin{subfigure}[b]{0.32\textwidth}
         \centering
         \includegraphics[width=0.92\textwidth]{figures/TIM_VGG_ensemble.png}
         \caption{TinyImageNet VGG Ensemble}
     \end{subfigure}\\
     \begin{subfigure}[b]{0.32\textwidth}
         \centering
         \includegraphics[width=0.92\textwidth]{figures/C10_RN34_ensemble.png}
         \caption{CIFAR-10 ResNet Ensemble}
     \end{subfigure}
     \hfill
     \begin{subfigure}[b]{0.32\textwidth}
         \centering
         \includegraphics[width=0.92\textwidth]{figures/C100_RN34_ensemble.png}
         \caption{CIFAR-100 ResNet Ensemble}
     \end{subfigure}
     \hfill
     \begin{subfigure}[b]{0.32\textwidth}
         \centering
         \includegraphics[width=0.92\textwidth]{figures/TIM_RN34_ensemble.png}
         \caption{TinyImageNet ResNet Ensemble}
     \end{subfigure}
     \caption{Analysis of ensemble diversity at difference temperatures}\label{fig:ensemble_analysis}
\end{figure}
